# Supplementary material for: Fast protein folding is governed by memory-dependent friction
Source: arXiv:2208.13842 ancillary file (2022-10-21)
Supplement: Supplementary file 1 [file SI_Document.pdf]

# Protein folding is governed by memory-dependent friction - Supplementary Information

Benjamin A. Dalton, Cihan Ayaz, Lucas Tepper, and Roland R. Netz
*Freie Universität Berlin, Fachbereich Physik, 14195 Berlin, Germany*

## CONTENTS


1. Simulations details and analysis 2
2. The generalised Langevin equation and memory-kernel extraction 3
3. Investigation of discretisation effects with alanine-9 homo-peptide chain 4
4. Position-dependent friction 6
5. Evaluating Markovian mean first-passage times - position-dependent and -independent friction 8
6. Free energy profiles for eight proteins in the fraction of native contacts reaction coordinate 9
7. Memory kernels for eight proteins in the fraction of native contacts reaction coordinate 10
8. Parametrized heuristic curves for each protein 12
9. Comparison of various reaction coordinates 13
10. Prediction errors for barrier crossing times 15

References 16


## 1. SIMULATIONS DETAILS AND ANALYSIS

All simulation data presented in the main manuscript was provided by the group of David E. Shaw and was originally published by Lindorff-Larsen *et. al.* [1]. Simulations were performed using the Anton special purpose computer [2], using a modified CHARMM force-field [3], and a modified TIP3P water model. All simulations were performed with an integration time step $dt = 2.5$ fs, however, protein configurations were saved to file every 200 ps, significantly reducing the time resolution of the trajectory data relative to the simulation time discretization. Effects due to low time-resolution discretization are discussed in the Section 3. Here, we only consider 8 out of the 12 proteins presented in the original publication. Of the remaining four proteins, the BBL, Protein B, and Homeodomain do not exhibit distinct energy barriers separating folded and unfolded states when observed with the fraction of native contacts reaction coordinate. The BBA protein does exhibit a separation barrier, however, it is so low as to be negligible. For this reason, we neglect these four proteins in our analysis. All proteins were simulated at a unique temperature, identified as the appropriate melting temperature, and chosen to maximize the number of folding and unfolding events. In Table I, we show various relevant system parameters, including the total simulation time for each protein $t_{\mathrm{sim}}$, the simulation temperature $T$, the number of amino acid residues $N$, the total number of folding events $N_{\mathrm{f}}$ and unfolding events $N_{\mathrm{u}}$, all of which appear in the original publication. Additionally, we show properties of the free energy barriers, including the barrier heights faced by the folded and unfolded states, $U_0^{\mathrm{f}}$ and $U_0^{\mathrm{u}}$, the distances from the unfolded and folded states minima to the barrier tops, $L_0^{\mathrm{f}}$ and $L_0^{\mathrm{u}}$, and the effective reaction coordinate mass $m$.

In Table II, we show a range of time scales measured in our analysis. These include the memory times $\tau_{\mathrm{mem}}$, inertial times $\tau_{\mathrm{m}}$, diffusion times in the folded and unfolded domains, $\tau_{\mathrm{D}}^{\mathrm{f}}$ and $\tau_{\mathrm{D}}^{\mathrm{u}}$, the folding and unfolding mean first-passage

TABLE I. Table of relevant system parameters and measurements

| | $t_{\mathrm{sim}}$ [$\mu$s] | $T[K]$ | $N$ | $N_{\mathrm{f}}$ | $N_{\mathrm{u}}$ | $U_0^{\mathrm{f}}$ [$k_{\mathrm{B}}T$] | $U_0^{\mathrm{u}}$ [$k_{\mathrm{B}}T$] | $L_{\mathrm{u}}$ | $L_{\mathrm{f}}$ | $m$ ($\times 10^3$) [$u$] |
|---|---|---|---|---|---|---|---|---|---|---|
| Chignolin | 106 | 300 | 10 | 39 | 38 | 6.0 | 1.6 | 0.042 | 0.53 | 0.17 |
| Trp-Cage | 208 | 290 | 20 | 12 | 12 | 3.9 | 3.1 | 0.075 | 0.22 | 0.31 |
| Villin | 125 | 360 | 35 | 34 | 34 | 2.0 | 1.6 | 0.043 | 0.17 | 0.62 |
| WW Domain | 1137 | 360 | 35 | 12 | 11 | 6.3 | 2.7 | 0.14 | 0.29 | 0.77 |
| NTL9 | 2936 | 355 | 39 | 17 | 14 | 6.7 | 2.3 | 0.16 | 0.23 | 1.9 |
| Protein-G | 1154 | 350 | 56 | 12 | 13 | 4.5 | 2.3 | 0.10 | 0.16 | 2.3 |
| $\alpha_3$D | 707 | 370 | 73 | 12 | 12 | 3.2 | 1.7 | 0.090 | 0.14 | 3.4 |
| $\gamma$-Repressor | 643 | 350 | 80 | 10 | 12 | 2.1 | 2.1 | 0.047 | 0.24 | 3.7 |

TABLE II. Table of relevant extracted from MD trajectories. All time scales are given in units of $\mu$s.

| | $\tau_{\mathrm{mem}}$ | $\tau_{\mathrm{m}}$ ($\times 10^{-5}$) | $\tau_{\mathrm{D}}^{\mathrm{f}}$ | $\tau_{\mathrm{D}}^{\mathrm{u}}$ | $\tau_{\mathrm{MFP}}^{\mathrm{MD,f}}$ | $\tau_{\mathrm{MFP}}^{\mathrm{MD,u}}$ | $\tau_{\mathrm{MTP}}^{\mathrm{f}}$ ($\times 10^{-2}$) | $\tau_{\mathrm{MTP}}^{\mathrm{u}}$ ($\times 10^{-2}$) |
|---|---|---|---|---|---|---|---|---|
| Chignolin | 0.042 | 5.4 | 0.002 | 0.31 | 0.36 | 0.11 | 1.1 | 0.06 |
| Trp-Cage | 0.35 | 0.46 | 0.15 | 1.3 | 8.0 | 0.81 | 2.0 | 0.60 |
| Villin | 0.072 | 1.2 | 0.033 | 0.50 | 1.2 | 0.06 | 2.7 | 0.20 |
| WW Domain | 4.2 | 0.24 | 2.1 | 9.0 | 33.1 | 54.9 | 4.9 | 3.1 |
| NTL9 | 0.44 | 0.48 | 3.4 | 7.1 | 23.6 | 116.0 | 1.2 | 6.6 |
| Protein-G | 0.33 | 0.32 | 2.4 | 6.4 | 23.4 | 16.4 | 12.0 | 8.3 |
| $\alpha_3$D | 3.7 | 0.15 | 5.9 | 15.5 | 39.4 | 22.8 | 16.0 | 6.9 |
| $\gamma$-Repressor | 0.19 | 0.48 | 0.57 | 15.1 | 31.9 | 0.91 | 108.0 | 1.3 |

times $\tau_{\mathrm{MFP}}^{\mathrm{MD,f}}$ and $\tau_{\mathrm{MFP}}^{\mathrm{MD,u}}$ measure from MD simulations, and measured folding and unfolding mean transition-path times $\tau_{\mathrm{MTP}}^{\mathrm{f}}$ and $\tau_{\mathrm{MTP}}^{\mathrm{u}}$.

## 2. THE GENERALISED LANGEVIN EQUATION AND MEMORY-KERNEL EXTRACTION

For each protein, we project the all-atom trajectories onto the fraction of native contacts reaction coordinate $Q(t)$ and hence describe the trajectory of $Q(t)$ in terms of an approximate 1D GLE:

$$m\ddot{Q}(t) = -\int_0^t \Gamma(t-t')\dot{Q}(t')dt' - \nabla U\big[Q(t)\big] + F_R(t), \tag{S1}$$

The GLE is approximate in the sense that the memory kernels $\Gamma(t)$ are independent of position, as described in a recent publication [4]. $F_R(t)$ is the random force term, which has a zero mean $\langle F_R(t)\rangle = 0$, and satisfies the fluctuation-dissipation theorem $\langle F_R(t)F_R(t')\rangle = k_{\mathrm{B}}T\Gamma(t-t')$. $U(Q)$ is the potential of mean force, which is extracted uniquely for each protein according to $U(Q) = -k_{\mathrm{B}}T\log\big[\rho(Q)\big]$, where $\rho(Q)$ is the probability density over $Q(t)$. The total friction on a reaction coordinate is given by the converged plateau value of the integrated memory kernel:

$$\gamma = G(t\to\infty) = \int_0^\infty \Gamma(t)dt, \tag{S2}$$

where $G(t) = \int_0^t \Gamma(t')dt'$ is the running integral of the memory kernel.

To extract $\Gamma(t)$ for each system, we use the running integral extraction scheme for generalized potentials. The details of this extraction scheme can be found in references [5] and [6]. In short, we correlate Eq. S1 with the initial position of the reaction coordinate $Q(0)$:

$$m\Big\langle Q(0)\ddot{Q}(t)\Big\rangle = -\int_0^t \Big\langle \Gamma(t-t')Q(0)\dot{Q}(t')dt'\Big\rangle - \Big\langle Q(0)\nabla U\big[Q(t)\big]\Big\rangle + \Big\langle Q(0)F_R(t)\Big\rangle, \tag{S3}$$

and with the initial velocity of the reaction coordinate $\dot{Q}(0)$:

$$m\Big\langle \dot{Q}(0)\ddot{Q}(t)\Big\rangle = -\int_0^t \Big\langle \Gamma(t-t')\dot{Q}(0)\dot{Q}(t')dt'\Big\rangle - \Big\langle \dot{Q}(0)\nabla U\big[Q(t)\big]\Big\rangle + \Big\langle \dot{Q}(0)F_R(t)\Big\rangle, \tag{S4}$$

Due to the original orthogonality relations used to derive the GLE in Eq. S1, both $\big\langle Q(0)F_R(t)\big\rangle = 0$ and $\big\langle \dot{Q}(0)F_R(t)\big\rangle = 0$. Otherwise, we can write Eqs. S3 and S4 in terms of the position-velocity and velocity-velocity correlation functions $C^{Q\dot{Q}}(t) = \big\langle Q(0)\dot{Q}(t)\big\rangle$ and $C^{\dot{Q}\dot{Q}}(t) = \big\langle \dot{Q}(0)\dot{Q}(t)\big\rangle$, respectively, as well as the correlations between the reaction coordinate and the PMF gradients $C^{Q\nabla U}(t) = \big\langle Q(0)\nabla U\big[Q(t)\big]\big\rangle$, and the velocity of the reaction coordinate and the PMF gradients $C^{Q\nabla U}(t) = \big\langle \dot{Q}(0)\nabla U\big[Q(t)\big]\big\rangle$:

$$m\frac{d}{dt}C^{Q\dot{Q}}(t) = -\int_0^t \Gamma(t')C^{Q\dot{Q}}(t-t')dt' - C^{Q\nabla U}(t), \tag{S5}$$

$$m\frac{d}{dt}C^{\dot{Q}\dot{Q}}(t) = -\int_0^t \Gamma(t')C^{\dot{Q}\dot{Q}}(t-t')dt' - C^{\dot{Q}\nabla U}(t). \tag{S6}$$

We integrate Eq. S6 in the time domain and obtain an equation in terms of $G(t) = \int_0^t \Gamma(t')dt'$:

$$mC^{\dot{Q}\dot{Q}}(t) - mC^{\dot{Q}\dot{Q}}(0) = -\int_0^t G(t-t')C^{\dot{Q}\dot{Q}}(t'')dt'' + C^{Q\nabla U}(t) - C^{Q\nabla U}(0). \tag{S7}$$

Using the identity that $\frac{d}{dt}C^{Q\dot{Q}}(t) = C^{Q\ddot{Q}}(t) = -C^{\dot{Q}\dot{Q}}(t)$, which can be confirmed using integration by parts, we evaluate Eq. S5 at t=0, and obtain $mC^{\dot{Q}\dot{Q}}(0) = C^{Q\nabla U}(0)$. It follows that:

$$\frac{C^{\dot{Q}\dot{Q}}(t)}{C^{\dot{Q}\dot{Q}}(0)}C^{Q\nabla U}(0) = C^{Q\nabla U}(t) - \int_0^t G(t-t')C^{\dot{Q}\dot{Q}}(t'').dt'' \tag{S8}$$

Eq. S8 can be discretized using the trapezoidal rule for numerical integration. Using $G(0) = 0$, we arrive at the following numerical extraction scheme, which we use to extract the discrete representation of $G(t)$ directly from the trajectory of a given reaction coordinate:

$$G_i = \begin{cases} 0, & i = 0 \\ \frac{2}{\Delta t C_0^{\dot{Q}\dot{Q}}}\left[C_1^{\nabla UQ} - \frac{C_0^{\nabla UQ}}{C_0^{\dot{Q}\dot{Q}}}C_1^{\dot{Q}\dot{Q}}\right], & i = 1 \\ \frac{2}{\Delta t C_0^{\dot{Q}\dot{Q}}}\left[C_i^{\nabla UQ} - \frac{C_0^{\nabla UQ}}{C_0^{\dot{Q}\dot{Q}}}C_i^{\dot{Q}\dot{Q}} - \Delta t\sum_{j=1}^{i-1} G_j C_{i-j}^{\dot{Q}\dot{Q}}\right], & i > 1 \end{cases} \tag{S9}$$

$C_i^{\dot{Q}\dot{Q}}$ and $C_i^{\nabla UQ}$ are the discretized representations of the velocity-velocity correlation function and the correlations between the reaction coordinate and the gradients of the PMF, respectively.

## 3. INVESTIGATION OF DISCRETISATION EFFECTS WITH ALANINE-9 HOMO-PEPTIDE CHAIN

The data analysed in this paper are only available in low time resolution. The original simulations were performed with time steps $dt$ =2.5 fs, however, the protein configurations are saved at time intervals of $\Delta t$ =0.2 ns. Thus, six orders of magnitude of time resolution are not accessible for our analysis. To investigate the extent to which this low-resolution representation of the data can yield reliable results, we consider a system for which we have full-time-resolution data, over long simulation times. Having access to such data, we systematically discretize over a range of sub-sampled time steps $\Delta t$. We use a previously published trajectory of the 9-residue homo-alanine peptide ($Ala_9$) [5] and investigate the deviation in the accuracy of the memory time $\tau_{\text{mem}}$ incurred as a result of decreasing time resolution. The $Ala_9$ system is simulated using Gromacs with the Amber03 force field, and 4023 explicit SPC/E water molecules. The simulation time step is $dt = 1$ fs and total simulation time is 10 $\mu$s. For a reaction coordinate, we use the standard $HB_4$ for $\alpha$-helix forming chains, which is given by the average of the separation between the $n^{\text{th}}$ residue nitrogen and $n^{\text{th}}$+4 residue oxygen, for $n$ = 2, 3, and 4.

We generate low-resolution trajectories by evenly sub-sampling at $\Delta t$ = 0.01, 0.1, 1, 10, 100, and 200 ps intervals. We then extract the running integrals of the memory kernels (as described in Section 2) for each discretization. In Fig. S1A, we show the running integrals G($t$) for the fully resolved data ($\Delta t$ = 0.001 ps) and four other discretizations. The corresponding $\Gamma(t)$ functions are given in Fig. S1B. Note that the extracted G(t) function is remarkably unaffected by the discretization, up until $\Delta t$ = 10 ps. For $\Delta t$ >10 ps, we incur numerical oscillations in G(t). To smooth out the oscillations in the memory kernels, the discrete values for the memory kernels are evaluated by $\Gamma_i = (G_{i+1} - G_{i-1})/2\Delta t$. Due to the robust extraction of the G($t$) plateau-value, the extraction method yields accurate zero-frequency friction $\gamma$ over the full range of discretization. This is clear in Fig. S1C. Here, we compare $\gamma$ evaluated in two ways. In the first, we fit a single-component exponential function to the long-time tail of $\Gamma(t)$ and hence replace the noisy long-time-tail data with the clean fit. We then revert this $\Gamma(t)$ back to a running integral and hence take the long-time limit of the running integral as $\gamma$. In the second method, we evaluate the average of the originally-extracted running integral (no exponential fit) over the plateau region for $t$ > 2000 ps. This first method is representative of how we evaluate $\gamma$ in the main manuscript. This second method is purely complementary and provides an error estimate, taken as

the standard deviations over the same range. Both methods are in agreement. The importance of Fig. S1C should not be understated. It tells us that even under such low resolution, we can accurately evaluate the zero-frequency friction using kernel extraction techniques. Thus we have a robust method for evaluating the friction on a reaction coordinate, which is suitable for low-time resolution data.

Finally, in Fig. S1D, we show the memory times $\tau_{\text{mem}} = \int_0^\infty t\Gamma(t)dt / \int_0^\infty \Gamma(t)dt$, as a function of the discretization steps size. We express the data as a percentage of the memory time, as evaluated for the fully resolved trajectory $\tau_{\text{mem}}(\Delta t = 1fs)$. We rescale the discretization steps-size also by $\tau_{\text{mem}}(\Delta t = 1fs)$, which provides an approximation of the relative error expected for a discretised system, given the intrinsic memory time of the corresponding fully-resolved system. In the case of the 8 fast-folding proteins, the corresponding fully-resolved system is the simulation with step size 2.5 fs. Thus, we see that there is a 20% reduction in the accuracy of the memory times for time-series discretization spanning four orders of magnitude. For lower resolution discretizations, the accuracy drops more

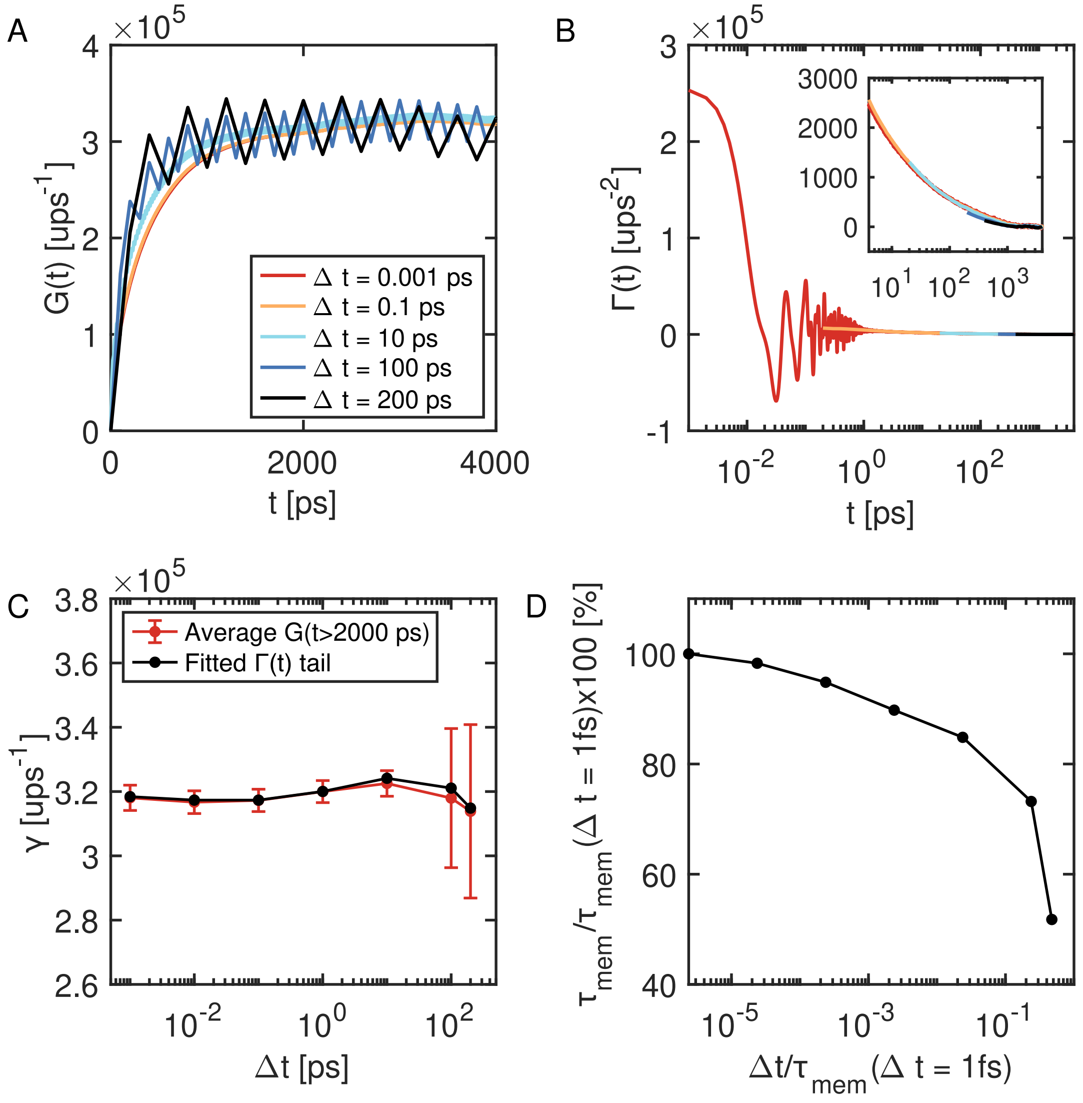


FIG. S1. $Ala_9$ discretization and memory time extraction. A) Memory kernel running integrals G($t$) extracted from $HB_4$ reaction coordinate trajectories at different time-series resolutions ($\Delta t$), with discretizations spanning five orders of magnitude. B) Corresponding memory kernels $\Gamma(t)$. The inset is a magnification of the long-time tail. C) Zero-frequency friction on the $HB_4$ reaction coordinate, evaluated via the memory kernel extraction, as a function of discretization. The red points with error bars show the average of $G(t)$ for each discretization, taken in the range 2 $\mu$s $\leq$ t $\leq$ 4 $\mu$s. The error bars show the standard deviations. The black points show the plateau values for $G(t)$, taken as the running integral of $\Gamma(t)$, with a fitted single exponential long-time tail. D) Memory times $\tau_{\text{mem}}$, evaluated via the 1st-moment method, as a function of rescaled discretization step size, expressed as a percentage of the memory time evaluated for the fully resolved data $\tau_\Gamma(\Delta t = 1\text{fs}) = 420$ ps.

rapidly. Given the range of memory times observed for the 8 proteins studied in this paper, we expect a range of $1{\times}10^{-5} < 0.2$ ns$/\tau_{\rm mem}(\Delta t = 2.5$ fs$) < 1{\times}10^{-3}$. Thus, we can suggest that the memory times presented in this paper, evaluated for the low-time-resolution trajectories, are inaccurate by at most 20%, which is a reassuring result.

## 4. POSITION-DEPENDENT FRICTION

In Eq. 3 of the main manuscript, we show an equation to predict barrier crossing times using memoryless constant friction. One can add position-dependent friction, such that:

$$\tau_{\rm MFP}^{\rm Mar}(Q_{\rm s}, Q_{\rm e}) = \beta \int_{Q_{\rm s}}^{Q_{\rm e}} \gamma(x) {\rm e}^{\beta U(x)} \left[ \int_{-\infty}^{x} {\rm e}^{-\beta U(y)} dy \right] dx, \tag{S10}$$

where the superscript *Mar* indicates that this is a purely Markovian prediction. Written in this way, with comma-separated arguments $\tau_{\rm MFP}^{\rm Mar}(Q_{\rm s}, Q_{\rm e})$, we indicate that $\tau_{\rm MFP}^{\rm Mar}$ is a profile, with a fixed start-point $Q_{\rm s}$ and a variable end-point $Q_{\rm e}$. The quantity $\tau_{\rm MFP}^{\rm Mar}(Q_{\rm s}, Q_{\rm e})$ can be extracted from the $Q(t)$ trajectories for each protein, where $Q_{\rm s}$, and $Q_{\rm e}$ are appropriately chosen for both folding and unfolding processes. Note that here we describe a convention suitable for folding processes. To evaluate unfolding profiles, the free energy and friction must be reflected on the $Q$-axis. Having extracted $\tau_{\rm MFP}^{\rm Mar}(Q_{\rm s}, Q_{\rm e})$, we can evaluate $\gamma(Q_{\rm e})$ in both the folding and unfolding directions. Using the identity $\partial[\int_x^y f(z)dz]/\partial y = f(y)$, we take the derivative of Eq. S10 with respect to $Q_{\rm e}$:

$$\frac{\partial \tau_{\rm MFP}^{\rm Mar}(Q_{\rm s}, Q_{\rm e})}{\partial Q_{\rm e}} = \beta \gamma(Q_{\rm e}) {\rm e}^{\beta U(Q_{\rm e})} \left[ \int_{Q_0}^{Q_{\rm e}} {\rm e}^{-\beta U(y)} dy \right], \tag{S11}$$

which we then solve for $\gamma(Q_{\rm e})$:

$$\gamma(Q_{\rm e}) = \frac{1}{\beta Z_{\rm e}} \frac{\partial \tau_{\rm MFP}^{\rm Mar}(Q_{\rm s}, Q_{\rm e})}{\partial Q_{\rm e}} {\rm e}^{-\beta U(Q_{\rm e})} \tag{S12}$$

where $Z_{\rm e}$ is given by:

$$Z_{\rm e} = \int_{Q_0}^{Q_{\rm e}} {\rm e}^{-\beta U(y)} dy, \tag{S13}$$

and $Q_0$ is the left-bound of the free-energy profile.

In Figs. S2A and 1B, we show $\gamma(Q_{\rm e})$, evaluated in both the folding and unfolding directions, for two example proteins. The friction profiles are evaluated between the folded and unfolded state minima, as indicated by the free-energy profile overlaid on the figures. We see that, according to the Markovian model Eq. S10, the friction experienced by each protein as it folds is different from that experienced when unfolding. This was already shown to be the case for the 9-residue alanine homo-peptide [5]. It was stated there that there is no fully-consistent way to describe the folding and unfolding dynamics using a Markovian model. We emphasis that here by reconstructing the barrier-crossing-time profiles for folding and unfolding while permuting the friction. Using Eqs. S18 and S19 below, we can reproduce the folding and unfolding time profiles with the corresponding extracted friction profiles (Figs. S2C and 1D). This is to be expected and acts as a consistency check. However, we can not predict the folding times across $Q$ using the unfolding friction. This result validates that there is no consistent way to predict folding kinetics with a position-dependent Markovian model since there is no single, unique friction profile belonging to the reaction coordinate.

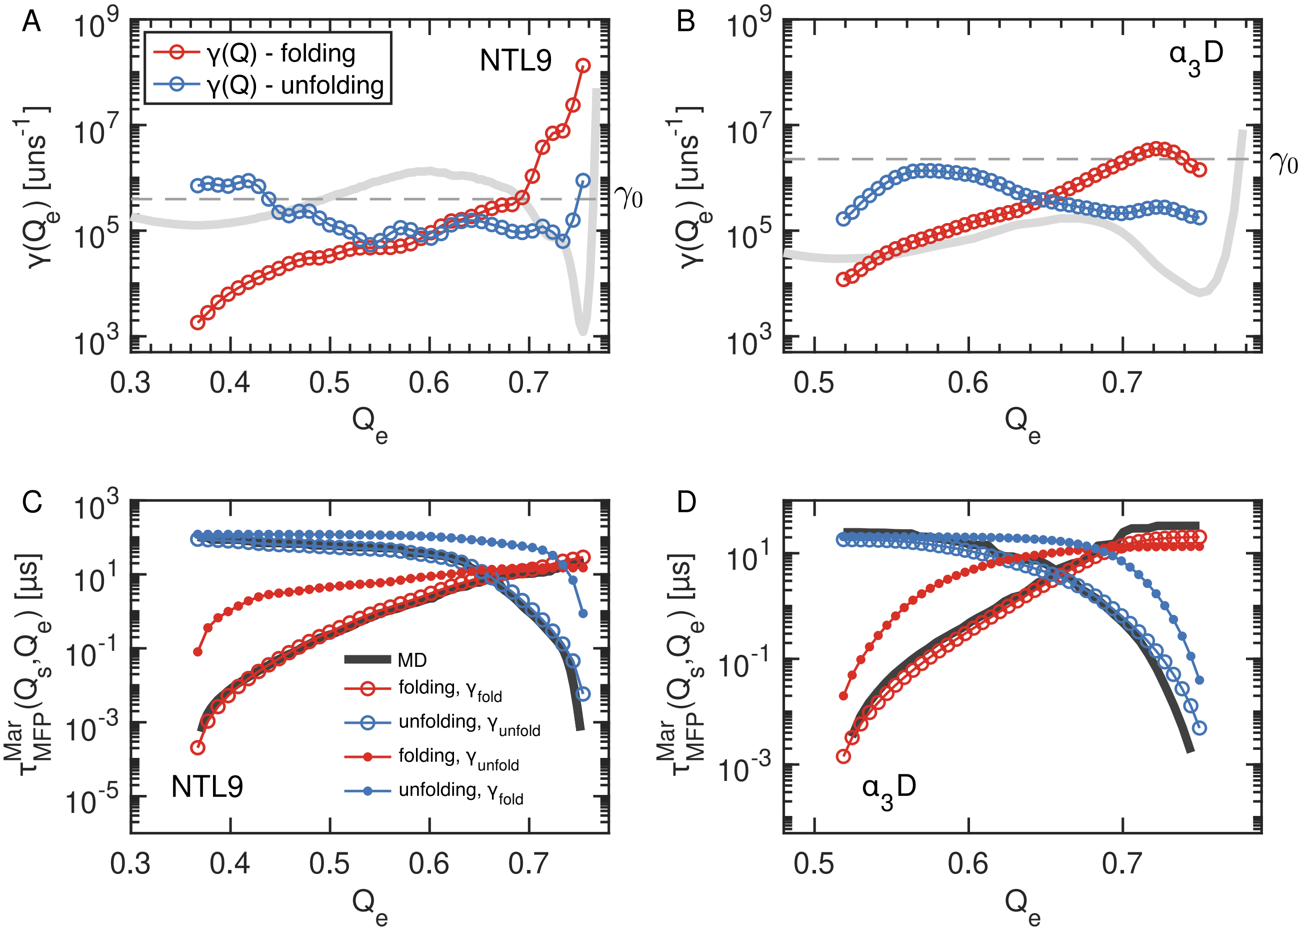


FIG. S2. Position-dependent friction depends on the folding direction. A) and B) show the reaction coordinate position dependence of memoryless friction, calculated for either the folding (red) or unfolding (blue) direction, for the NTL9 and $\alpha_3$D proteins, respectively. $Q_\mathrm{s}$ is the start-point of a transition, which we keep fixed, and $Q_\mathrm{e}$ is the end-point, which is the independent variable. The free-energy profile is overlaid in light gray, displaying the minima and barriers of interest. The dashed lines indicate the value of zero-frequency friction for each protein, as calculated in the main manuscript. C) and D) show various calculations of barrier crossing time profiles for the NTL9 and $\alpha_3$D proteins, respectively. The bold black lines show $\tau_{\mathrm{MFP}}(Q)$, extracted from the MD trajectories. The open circles show a validation calculation for reconstructing crossing-times with the corresponding $\gamma(Q)$ profiles from A) and B). The filled circles show an attempted construction of $\tau_{\mathrm{MFP}}(Q)$, using the anti-corresponding $\gamma(Q)$.

## 5. EVALUATING MARKOVIAN MEAN FIRST-PASSAGE TIMES - POSITION-DEPENDENT AND -INDEPENDENT FRICTION

For a purely Markovian system with constant friction, the mean first-passage time between reaction coordinate positions $Q_\mathrm{s}$ and $Q_\mathrm{e}$ is given by:

$$\tau_{\mathrm{MFP}}^{\mathrm{Mar}}(Q_\mathrm{s}|Q_\mathrm{e}) = \beta\gamma \int_{Q_\mathrm{s}}^{Q_\mathrm{e}} \mathrm{e}^{\beta U(x)} \left[ \int_{-\infty}^{x} \mathrm{e}^{-\beta U(y)} dy \right] dx \tag{S14}$$

where the subscript $s$ indicates a start position and $e$ indicates an end position. The bar-separator | indicates that we are not evaluating a profile across $Q$-space, as we did in the previous section (Eq. S10.). Rather, we are evaluating the passage time between two single points $Q_\mathrm{s}$ and $Q_\mathrm{e}$, which we choose to be the free energy minima and barrier tops. In practice, the inner integral will have a lower limit at the appropriate edge of the confining potential $Q_0$. The discrete form of the inner integral will therefore be:

$$\int_{-\infty}^{x} \mathrm{e}^{-\beta U(y)} dy \quad \rightarrow \quad \sum_{i=0}^{j} \mathrm{e}^{-\beta U(Q_i)} \Delta y \tag{S15}$$

The composite integral becomes:

$$\int_{Q_\mathrm{s}}^{Q_\mathrm{e}} \mathrm{e}^{\beta U(x)} \left[ \int_{-\infty}^{x} \mathrm{e}^{-\beta U(y)} dy \right] dx \rightarrow \sum_{j=a}^{b} \mathrm{e}^{\beta U(Q_j)} \left[ \sum_{i=0}^{j} \mathrm{e}^{-\beta U(Q_i)} \Delta y \right] \Delta x. \tag{S16}$$

$\Delta x$ and $\Delta y$ are the discretization step sizes, set by the free-energy histogram. $a$ and $b$ are the indices for the bins located at the beginning and the end of the transition, which might be, for example, the unfolded state minimum and the barrier top, respectively, for a folding transition. Since the bin size is fixed, the two discretization step sizes are equal $\Delta x = \Delta y$, which we just write as $\Delta Q$. The discrete form of the exact mean passage time is then:

$$\tau_{\mathrm{MFP}}^{\mathrm{Mar}}(Q_\mathrm{s}|Q_\mathrm{e}) = \beta\gamma\Delta Q^2 \sum_{j=a}^{b} \sum_{i=0}^{j} \mathrm{e}^{\beta U(Q_j)} \mathrm{e}^{-\beta U(Q_i)}. \tag{S17}$$

For the case of position-dependent friction, outlined in Eq. S10, $\gamma(Q)$ resides inside the outer integral, such that the composite integral becomes:

$$\tau_{\mathrm{MFP}}^{\mathrm{Mar}}(Q_\mathrm{s}|Q_\mathrm{e}) = \int_{Q_\mathrm{s}}^{Q_\mathrm{e}} \gamma(x) \mathrm{e}^{\beta U(x)} \left[ \int_{-\infty}^{x} \mathrm{e}^{-\beta U(y)} dy \right] dx \rightarrow \sum_{j=a}^{b} \gamma_j \mathrm{e}^{\beta U(Q_j)} \left[ \sum_{i=0}^{j} \mathrm{e}^{-\beta U(Q_i)} \Delta y \right] \Delta x \tag{S18}$$

The discrete form is then written:

$$\tau_{\mathrm{MFP}}^{\mathrm{Mar}}(Q_\mathrm{s}|Q_\mathrm{e}) = \beta\Delta Q^2 \sum_{j=a}^{b} \sum_{i=0}^{j} \gamma_j \mathrm{e}^{\beta U(Q_j)} \mathrm{e}^{-\beta U(Q_i)}. \tag{S19}$$

## 6. FREE ENERGY PROFILES FOR EIGHT PROTEINS IN THE FRACTION OF NATIVE CONTACTS REACTION COORDINATE

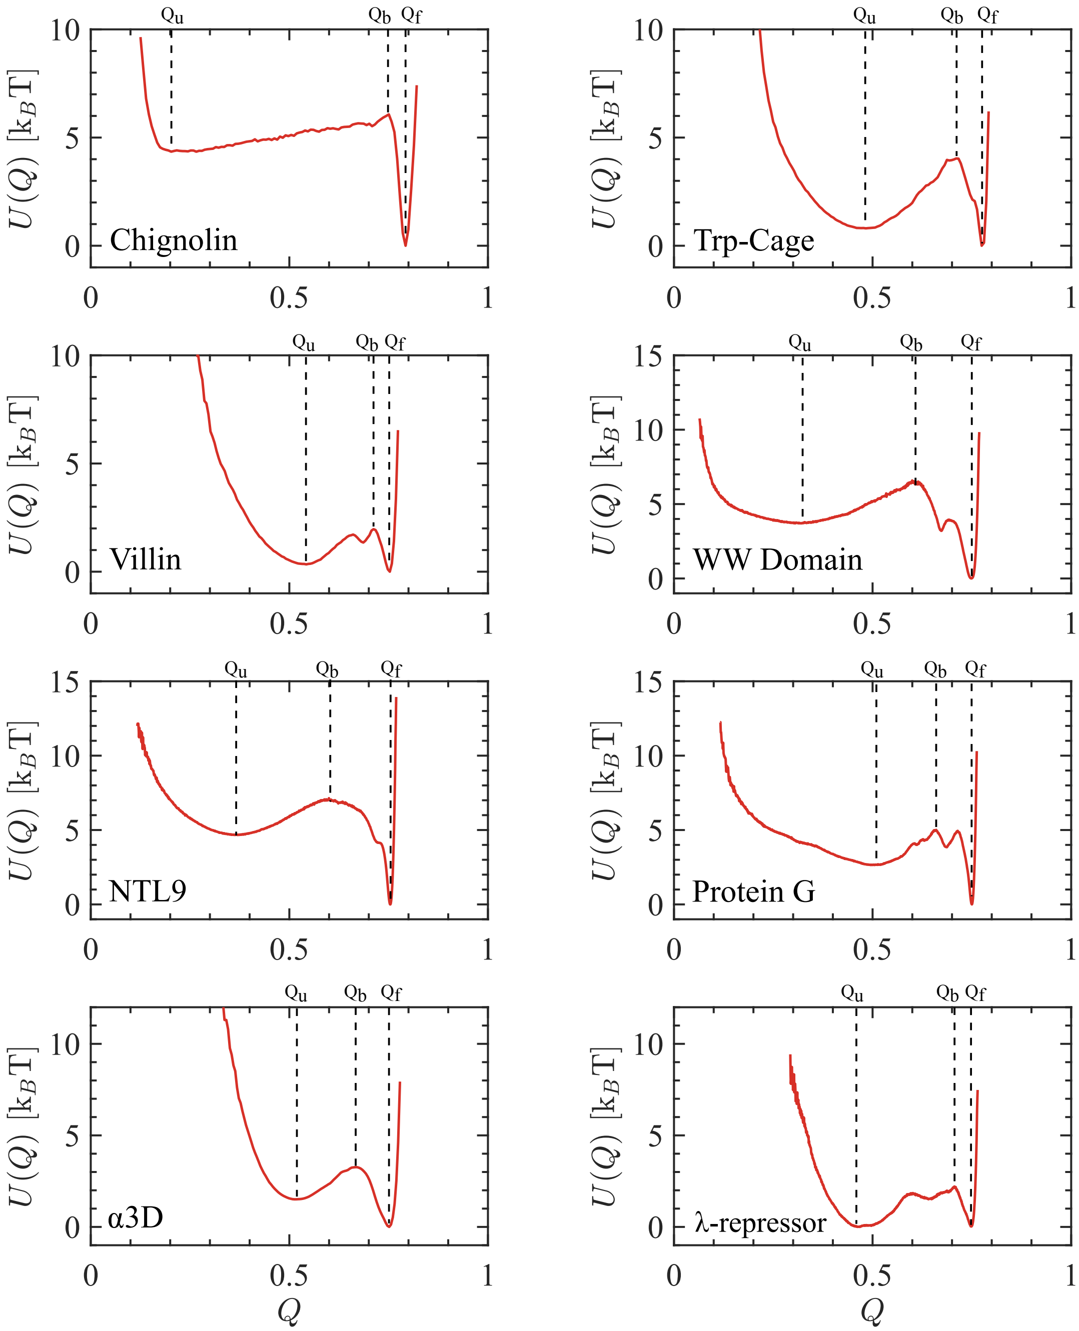


FIG. S3. Free energy profiles for the fraction of native contacts reaction coordinate, evaluated for the eight proteins. The unfolded $Q_{\mathrm{u}}$, barrier $Q_{\mathrm{b}}$, and folded $Q_{\mathrm{f}}$ states are indicated for each protein. Free energy profiles are calculated such that $U(Q) = -k_{\mathrm{B}}T\log[\mathrm{p(Q)}]$, where $p(Q)$ is the probability density for a given trajectory. Probability densities are calculated using normalised histograms, with 750 bins between $Q_{\mathrm{min}}$ and $Q_{\mathrm{max}}$ for each protein.

## 7. MEMORY KERNELS FOR EIGHT PROTEINS IN THE FRACTION OF NATIVE CONTACTS REACTION COORDINATE

Memory kernels for each protein are extracted for the fraction of native contacts reaction coordinate using the method given in Eq. S9. The results for the extractions are shown in Fig. S4. We expect that, due to the intrinsically low time resolution of the MD data, there exist decay modes that cannot be resolved by our extraction methods.

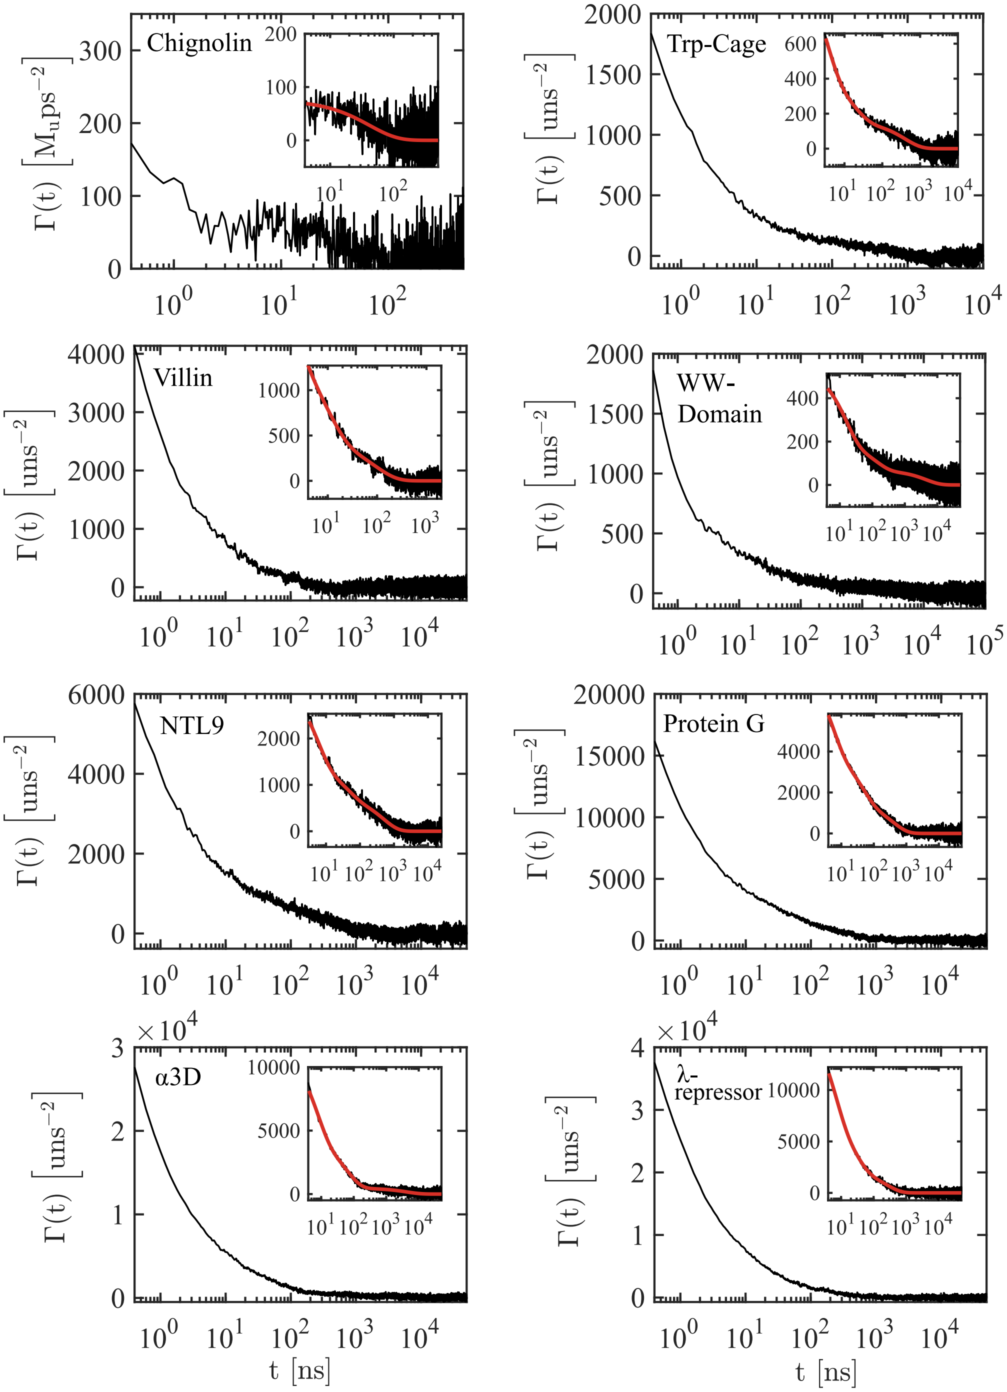


FIG. S4. Time-dependent memory kernels extracted via Eq. S9 for the 8 proteins. The main panel for each protein shows the full memory kernel. The inserts show the segment of the memory kernel that is used for the fit of the exponential series to the data, as well as the result for the fitting (red curve). For Chignolin, the exponential series contains two terms. For all other proteins, there are three terms in the series.

In the inset for each panel, we show results for a three-component exponential fit to the memory kernels, and the corresponding region of fitting (note that for the case of chignolin, we only fit two exponential components). The fitting parameters are shown in Table III, along with the zero-frequency friction $\gamma$ and the 1st-moment memory time $\tau_{\mathrm{mem}}$ for each protein. The zero-frequency friction can be reconstructed such that $\gamma = \sum_{i=1}^{M} \gamma_i$.

TABLE III. Table of fitting parameters for memory kernels of the eight proteins. Memory kernels are given by $\Gamma(t) = \sum_{i=1}^{M} \gamma_i \exp(-\mathrm{t}/\tau_\mathrm{i})/\tau_\mathrm{i}$, where $M = 2$ for Chignolin, and $M = 3$ for all other proteins. Time scales $\tau_i$ are given in units $\mu$s and amplitudes are in [uns$^{-1}$].

| | $\gamma_1$ ($\times 10^5$) | $\tau_1$ | $\gamma_2$ ($\times 10^3$) | $\tau_2$ ($\times 10^{-2}$) | $\gamma_3$ ($\times 10^3$) | $\tau_3$ ($\times 10^{-3}$) | $\gamma$ ($\times 10^5$) | $\tau_{\mathrm{mem}}$ |
|---|---|---|---|---|---|---|---|---|
| Chignolin | 0.0318 | 0.041 | 0.0798 | 0.01 | - | - | 0.032 | 0.042 |
| Trp-Cage | 0.609 | 0.39 | 4.8 | 1.7 | 2.22 | 2.9 | 0.68 | 0.36 |
| Villin | 0.408 | 0.092 | 10.5 | 0.95 | 2.2 | 1.4 | 0.53 | 0.072 |
| WW Domain | 2.98 | 4.5 | 16.1 | 13.0 | 5.1 | 10.6 | 3.2 | 4.21 |
| NTL9 | 3.55 | 0.49 | 28.7 | 4.2 | 10.1 | 3.3 | 3.9 | 0.45 |
| Protein-G | 5.88 | 0.41 | 113.5 | 4.3 | 22.4 | 2.8 | 7.3 | 0.33 |
| $\alpha_3$D | 19.6 | 4.3 | 239.0 | 6.3 | 53.6 | 4.9 | 22.6 | 3.73 |
| $\gamma$-Repressor | 5.42 | 0.26 | 148.5 | 2.8 | 60.3 | 2.2 | 7.6 | 0.19 |

## 8. PARAMETRIZED HEURISTIC CURVES FOR EACH PROTEIN

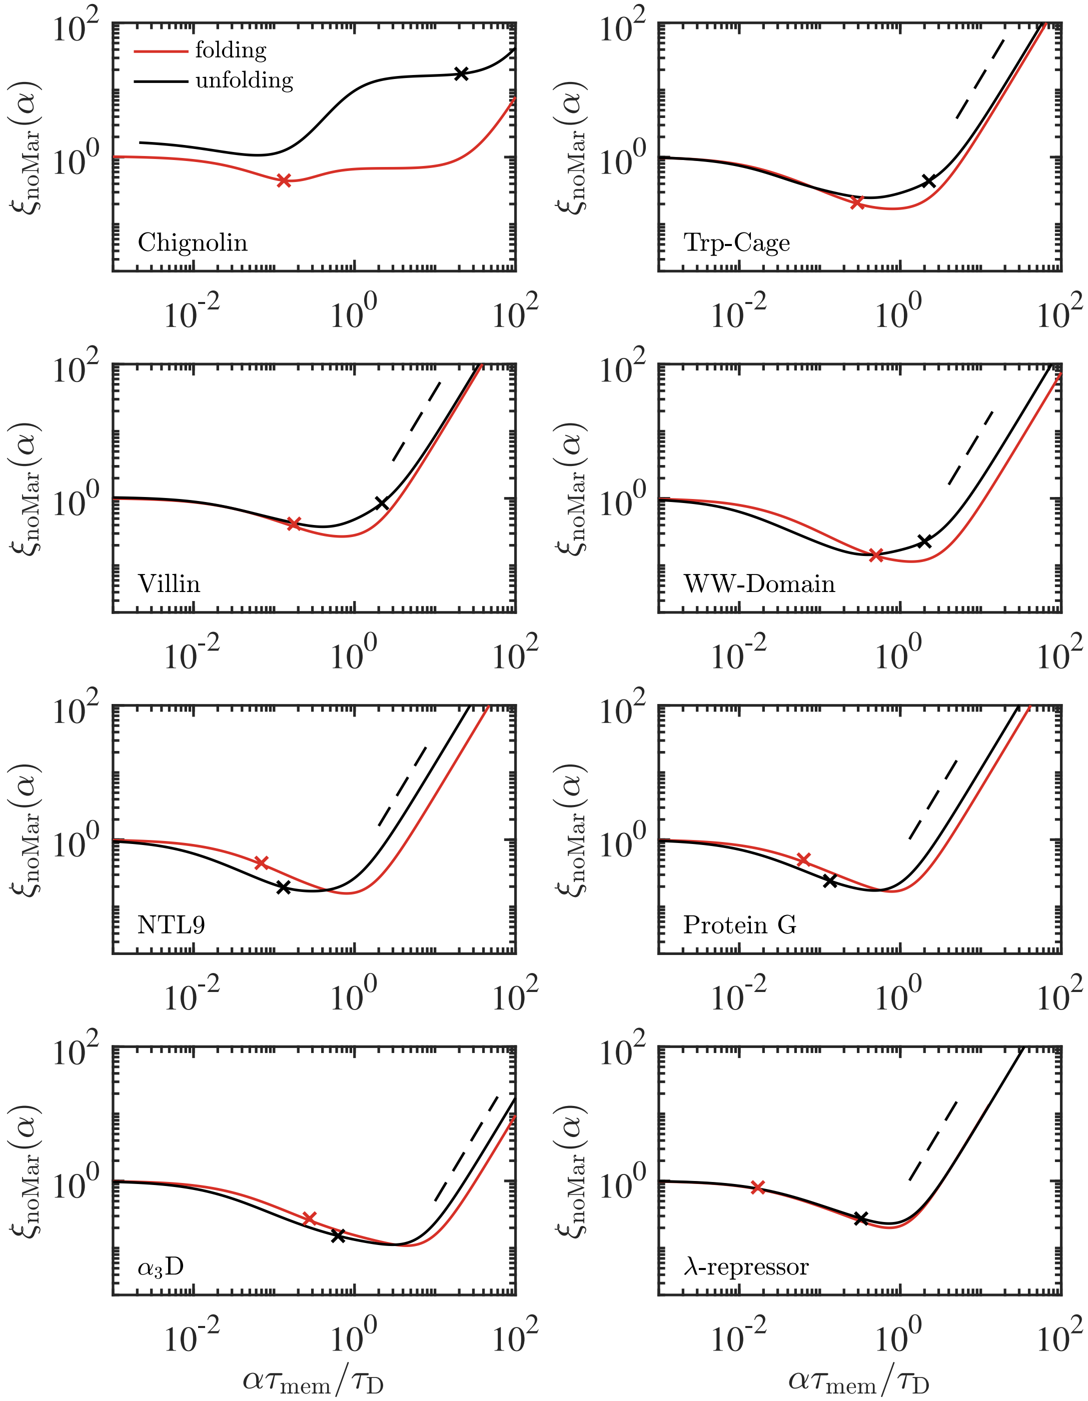


FIG. S5. Heuristic curves for folding and unfolding reactions. The three component heuristic curves, as given in Eqs. 3 and M2-M5 in the main text, are parametrised for each protein using values of $\tau_{\mathrm{D}}$, $\tau_{\mathrm{m}}$, $\tau_1$, $\tau_2$, $\tau_3$, $\gamma_1$, $\gamma_2$, $\gamma_3$, and $U_0$, plotted as a function of $\alpha\tau_{\mathrm{mem}}/\tau_{\mathrm{D}}$, by varying $\alpha$. All parameters are extracted directly from the MD simulations. The red and black crosses indicate the points on the curve where $\alpha = 1$, which corresponds to the value of $\xi_{\mathrm{noMar}}$ for a given protein. The heuristic predictions for the barrier crossing times $\tau^{H}_{\mathrm{MFP}}$ are rescaled by the over-damped, memoryless limit $\tau_{\mathrm{D}}\pi U_0 \mathrm{e}^{\beta U_0}/2\beta\sqrt{2}$.

## 9. COMPARISON OF VARIOUS REACTION COORDINATES

In the manuscript, we only consider the fraction of native contacts reaction coordinate $Q$. Alternative standard reaction coordinates for the analysis of MD protein simulation trajectories include:

1. the end-to-end distance ($R_{\rm e2e}$): the magnitude of the Cartesian vector separating the first and last $\alpha$-carbon atoms in a chain. For a chain of length $N$, the end-to-end distance is given by:

$$R_{\rm e2e}(t) = |\mathbf{r}_N(t) - \mathbf{r}_1(t)| \tag{S20}$$

2. the radius of gyration ($R_{\rm rgy}$): for a peptide chain with center of mass $\mathbf{r}_{\rm com}(t)$ and set of particle masses $m_i$, the radius of gyration is given by:

$$R_{\rm rgy}(t) = \sqrt{\frac{\sum_{i=1}^{N} m_i |\mathbf{r}_i(t) - \mathbf{r}_{\rm com}(t)|^2}{\sum_{i=1}^{N} m_i}}, \tag{S21}$$

where the summation is over all $N$ $\alpha$-carbon atoms.

3. the root-mean-squared deviation ($R^{\rm d}_{\rm rms}$): $\mathbf{r}^0_i$ is the position of the $i^{\rm th}$ $\alpha$-carbon in the native state (the native state is defined in the Materials and Methods). The root-mean-squared deviation for the configuration of a protein at time $t$, deviating from the native state, is given by:

$$R^{\rm d}_{\rm rms}(t) = \sqrt{\frac{1}{N}\sum_{i=1}^{N}\left(\tilde{\mathbf{r}}_i(t) - \mathbf{r}^0_i\right)^2}, \tag{S22}$$

where $\tilde{\mathbf{r}}_i(t)$ is the position vector of the $i^{\rm th}$ $\alpha$-carbon at time $t$, for a configuration that has been uniformly translated and rotated to minimize the RMS deviation from the native state.

4. the root-mean-squared pair-separation ($R^{\rm ps}_{\rm rms}$): $\mathbf{s}^0_{ij}$ is the pair-separation vector connecting the $i^{\rm th}$ and $j^{\rm th}$ residues in the native state, where $i$ and $j$ are indices from the native contacts list. $\mathbf{s}_{ij}(t) = \mathbf{r}_j(t) - \mathbf{r}_i(t)$ is the

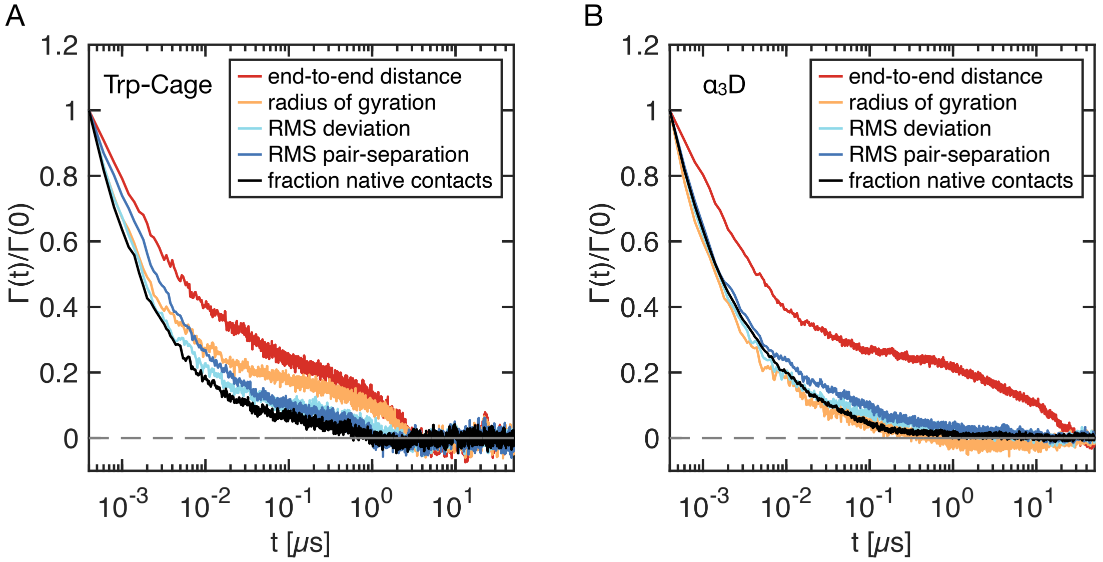


FIG. S6. Comparison of memory kernels for five different reaction coordinates. A) Memory kernels for Trp-Cage protein. Memory times, evaluated as the first moment of $\Gamma(t)$, are for $R_{\rm e2e}$, $R_{\rm rgy}$, $R^{\rm d}_{\rm rms}$, $R^{\rm ps}_{\rm rms}$, and $Q$, respectively: $\tau_{\rm mem} = 1.44\mu$s, $1.65\mu$s, $0.9\mu$s, $0.65\mu$s, and $0.48\mu$s . B) Memory kernels for $\alpha_3$D protein. Memory times are for $R_{\rm e2e}$, $R_{\rm rgy}$, $R^{\rm d}_{\rm rms}$, $R^{\rm ps}_{\rm rms}$, and $Q$, respectively: $\tau_{\rm mem} = 11.8\mu$s, $0.18\mu$s, $5.7\mu$s, $7.6\mu$s, and $2.9\mu$s .

pair-separation vector connecting the $i^{\text{th}}$ and $j^{\text{th}}$ residues at time $t$. $\mathbf{S}_{ij}(t,t') = \mathbf{s}_{ij}(t) - \mathbf{s}^0_{ij}$, then, is the time evolution of pair-separations, compared to native separations. The root-mean-squared pair-separation is given by:

$$R^{\text{ps}}_{\text{rms}}(t) = \sqrt{\frac{1}{N_l}\sum_{i,j}^{N_l}\left(s_{ij}(t) - s^0_{ij}\right)^2}, \tag{S23}$$

where $N_l$ is the number of residues in the list of native contacts and $s_{ij} = |\mathbf{s}_{ij}|$ is the magnitude of the a corresponding pair-separation vector.

The normalised memory kernels for these four reaction coordinates, plus the fraction of native contacts reaction coordinate $Q$ (described in the Materials and Methods), as shown in Fig. S6, reveal large variation, depending on the choice of the reaction coordinate, and on the protein. For the Trp-Cage protein, the fraction of native contacts reaction coordinate has the shortest memory time-scale, a factor of 3 less than the end-to-end distance, which has the longest. For the $\alpha_3$D protein, however, the radius of gyration memory kernel decays the fastest, two orders of magnitude faster than the end-to-end distance.

## 10. PREDICTION ERRORS FOR BARRIER CROSSING TIMES

We quantify the deviation for three theoretical predictions of the folding and unfolding times away from the measured values, across the full population of proteins. Considering the measured folding and unfolding times to be the target values $\tau^{\rm MD}_{{\rm MFP},i}$, and the theoretical prediction for each reaction time to be $\tau^{\rm theo}_{{\rm MFP},i}$, the absolute root-mean-square deviation (RMSD) for the full population, with folding and unfolding collected into a single set ($N = 16$), is given by:

$$\text{RMSD} = \sqrt{\frac{1}{N}\sum_{i=1}^{N}\left(\tau^{\rm MD}_{{\rm MFP},i} - \tau^{\rm theo}_{{\rm MFP},i}\right)^2} \tag{S24}$$

The distribution of $\tau^{\rm MD}_{{\rm MFP},i} - \tau^{\rm theo}_{{\rm MFP},i}$ for the three different theories, along with the corresponding RMSD values, is shown in Fig. S7A.

To logarithmically weight the deviations, as they appear in Fig. 3 of the main manuscript, we use the root-mean-square logarithmic deviation (RMSLD):

$$\text{RMSLD} = \sqrt{\frac{1}{N}\sum_{i=1}^{N}\left(\text{Log}(\tau^{\rm MD}_{{\rm MFP},i}) - \text{Log}(\tau^{\rm theo}_{{\rm MFP},i})\right)^2} \tag{S25}$$

The distributions of $\log(\tau^{\rm MD}_{\rm MFP,i}) - \log(\tau^{\rm theo}_{\rm MFP,i})$, for the three different theories, along with the corresponding RMSLD values, are shown in Fig. S7B.

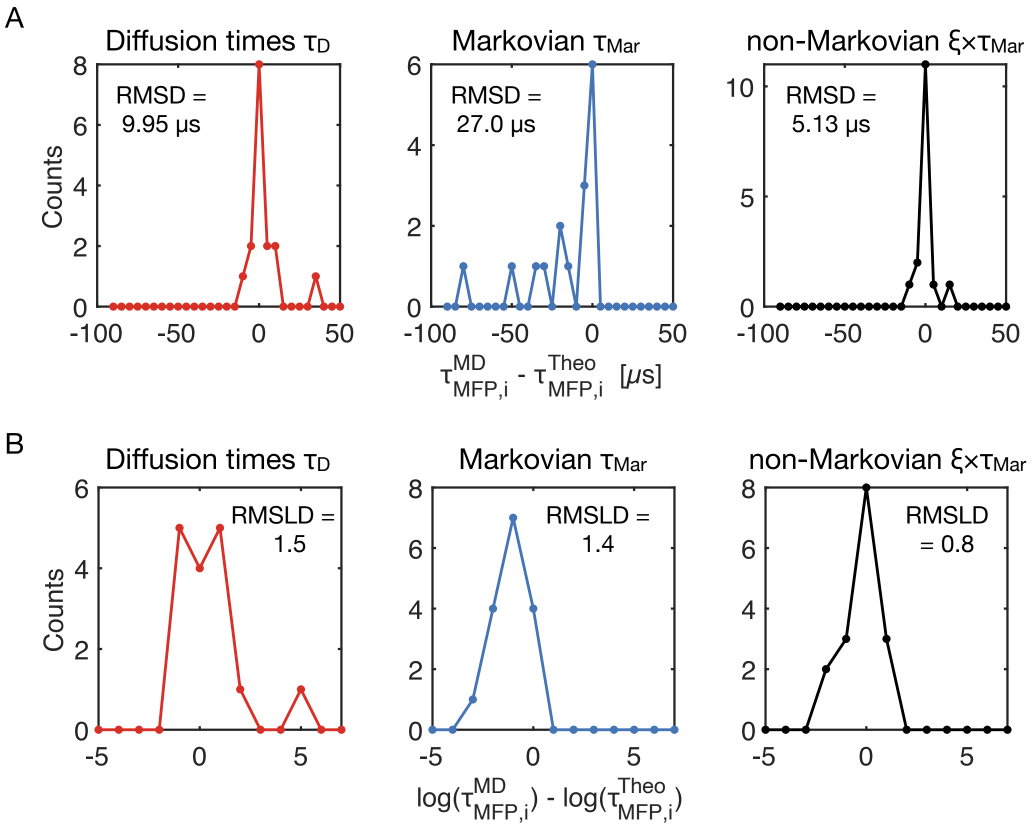


FIG. S7. Distributions for the deviations between theoretical predictions and measured values of the barrier crossing times. Folding and unfolding reactions are collected into a single set, such that $N = 16$. A) Root-mean-square deviations (RMSD) and B) the root-mean-square logarithmic deviations (RMSLD), revealing the logarithmically weighted spread of deviations.

[1] K. Lindorff-Larsen, S. Piana, R. O. Dror, and D. E. Shaw, Science **334**, 517 LP (2011).
[2] D. E. Shaw, R. O. Dror, J. K. Salmon, J. P. Grossman, K. M. Mackenzie, J. A. Bank, C. Young, M. M. Deneroff, B. Batson, K. J. Bowers, E. Chow, M. P. Eastwood, D. J. Ierardi, J. L. Klepeis, J. S. Kuskin, R. H. Larson, K. Lindorff-Larsen, P. Maragakis, M. A. Moraes, S. Piana, Y. Shan, and B. Towles, in *Proceedings of the Conference on High Performance Computing Networking, Storage and Analysis* (2009) pp. 1–11.
[3] S. Piana, K. Lindorff-Larsen, and D. E. Shaw, Biophysical journal **100**, L47 (2011).
[4] C. Ayaz, L. Scalfi, B. A. Dalton, and R. R. Netz, Physical Review E **105**, 54138 (2022).
[5] C. Ayaz, L. Tepper, F. N. Brünig, J. Kappler, J. O. Daldrop, and R. R. Netz, Proceedings of the National Academy of Sciences **118**, e2023856118 (2021).
[6] B. Kowalik, J. O. Daldrop, J. Kappler, J. C. F. Schulz, A. Schlaich, and R. R. Netz, Physical Review E **100**, 12126 (2019).
